# Supplementary material for: LATTEO: A Framework to Support Learning Asynchronously Tempered with Trusted Execution and Obfuscation
Source: arXiv:2502.04601 source file (2025-02-07)
Supplement: Supplementary file 1 [file appendixDefinition.tex]

\section{Computational Assumptions}
\label{app:definition}
Let $\mathbb{G}_{1}$ and $\mathbb{G}_{2}$ be two cyclic multiplicative groups of prime order $q$ generated by $g_1$ and $g_2$ respectively, $\hat{e}: \mathbb{G}_{1} \times \mathbb{G}_{2} \rightarrow \mathbb{G}_{T}$ be a bilinear map such that $\forall x \in \mathbb{G}_{1}, y \in \mathbb{G}_{2}$, and $a,b \in \mathbb{Z}_q$, $\hat{e}(x^{a},y^{b}) = \hat{e}(x,y)^{ab}$, and $\hat{e}(g_{1},g_{2}) \neq 1$. 

\begin{definition}%
\label{def:ddh}
The Decisional Diffie-Hellman (DDH) problem in prime order group $\mathbb{G}=<\hspace{-0.1cm}g\hspace{-0.1cm}>$ is defined as follows: on input $g$, $g^{a}$, $g^{b}$, $g^{c}$ $\in$ $\mathbb{G}$, decide if $c$ = $ab$ or $c$ is a random element of $\mathbb{Z}_{q}$.
\end{definition}

\begin{definition}%
\label{def:dbdh}
Let algorithm BDH\_Gen($1^{\lambda}$) output the parameters ($\hat{e}(\cdot,\cdot), q,g_{1},g_{2},\mathbb{G}_{1},\mathbb{G}_{2},\mathbb{G}_{T}$) where there is an efficiently computable isomorphism $\psi$ from $\mathbb{G}_{2}$ to $\mathbb{G}_{1}$. The Decisional Bilinear Diffie-Hellman (DBDH) problem is defined as follows: given $g_{1} \in \mathbb{G}_{1}$, $ g_{2},g^{a}_{2},g^{b}_{2},g^{c}_{2} \in \mathbb{G}_{2}$ and $Z \in \mathbb{G}_{T}$ as input, decide if $Z = \hat{e}(g_{1},g_{2})^{abc}$ or $\hat{e}(g_{1},g_{2})^{R}$ for $R \in \mathbb{Z}_{q}$.
\end{definition}

\begin{definition}%
\label{def:kddh}
The k-Decisional Diffie-Hellman Inversion (k-DDHI) problem in prime order group $\mathbb{G} = <\hspace{-0.1cm}g\hspace{-0.1cm}>$ is defined as follows: on input a (k+2)-tuple $ g,g^{s},g^{s^{2}}, \ldots,g^{s^{k}}, g^{u} \in \mathbb{G}^{k+2}$, decide if $u = 1/s$ or $u$ is a random element of $\mathbb{Z}_{q}$.
\end{definition}

\begin{definition}%
\label{def:xdh}
Let BDH\_Gen($1^{\lambda}$) output the parameters for a bilinear mapping $(\hat e) : \mathbb{G}_{1} \times \mathbb{G}_{2} \rightarrow \mathbb{G}_{T}$. The eXternal Diffie-Hellman (XDH) assumption states that, for all probabilistic polynomial time adversaries $\mathcal{A}$, the DDH problem is hard in $\mathbb{G}_{1}$. This implies that there does not exist an efficiently computable isomorphism $\psi^{\prime} : \mathbb{G}_{1} \rightarrow \mathbb{G}_{2}$.
\end{definition}
